# Supplementary material for: ColonNeRF: High-Fidelity Neural Reconstruction of Long Colonoscopy
Source: arXiv:2312.02015 source file (2024-03-21)
Supplement: Supplementary file 1 [file Supp.pdf]

## Supplementary Material

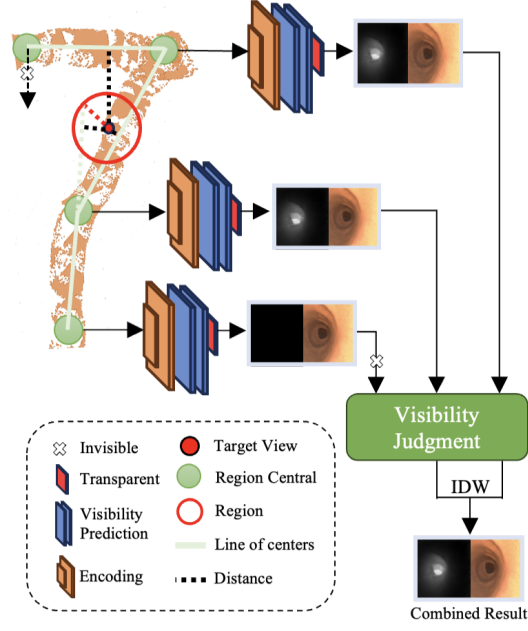

**Fig. 1.** Detailed depiction of intestinal seamless integration module.

**Table 1.** Ablation study about coarse-to-fine and fine-input which uses fine-grained data as input in the first stage.

|                | PSNR $\uparrow$ | VGG $\downarrow$ | ALEX $\downarrow$ | MS-SSIM $\uparrow$ |
|----------------|-----------------|------------------|-------------------|--------------------|
| Fine-input     | 26.23           | 0.3826           | 0.2488            | 0.8402             |
| Coarse-to-fine | <b>27.14</b>    | <b>0.364</b>     | <b>0.2214</b>     | <b>0.8611</b>      |

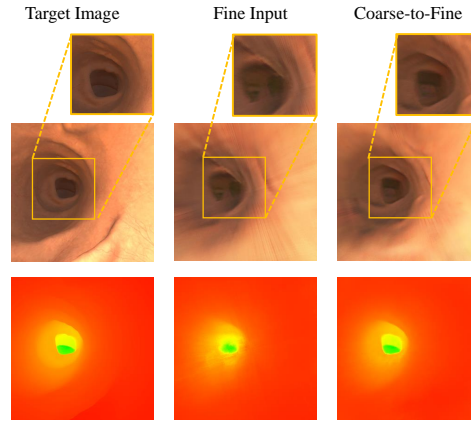

**Fig. 2.** Novel view synthesis from the coarse-to-fine and fine-input ways in the synthetic data.

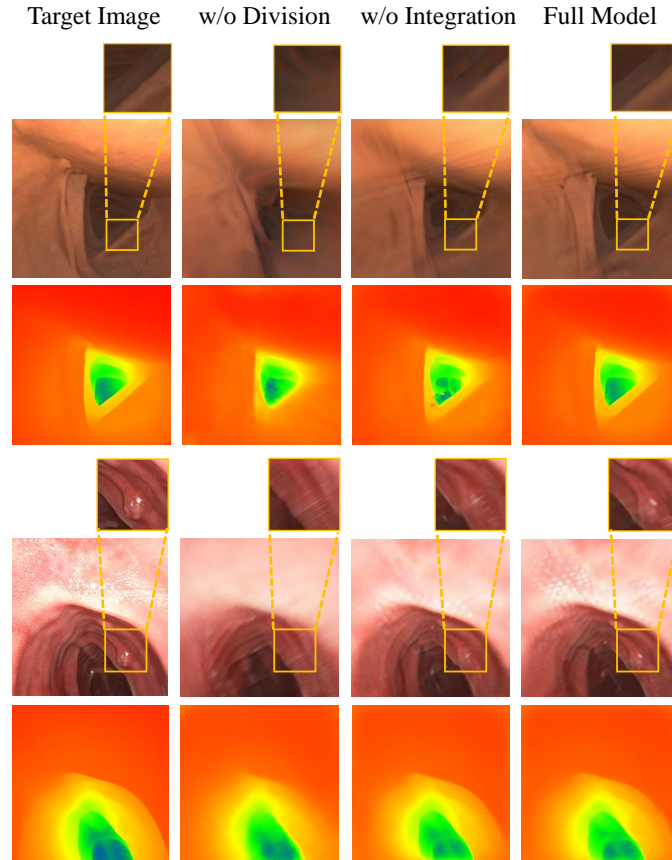

**Fig. 3.** Novel view synthesis without a region division module or integration module.
